# Supplementary material for: Surface charge theorem and topological constraints for edge states: An analytical study of one-dimensional nearest-neighbor tight-binding models
Source: arXiv:1911.06886 ancillary file (2020-04-05)
Supplement: Supplementary file 1 [file supp_paper_prb.pdf]

# Surface charge theorem and topological constraints for edge states: An analytical study of one-dimensional nearest-neighbor tight-binding models
# Supplemental Material

Mikhail Pletyukhov,[1] Dante M. Kennes,[1] Jelena Klinovaja,[2] Daniel Loss,[2] and Herbert Schoeller[1,*]

[1] *Institut für Theorie der Statistischen Physik, RWTH Aachen, 52056 Aachen, Germany and JARA - Fundamentals of Future Information Technology*

[2] *Department of Physics, University of Basel, Klingelbergstrasse 82, CH-4056 Basel, Switzerland*

(Dated: January 21, 2020)

The following appendices comprise the Supplemental Material to Ref. 1.

## I. PARAMETERS FOR THE FIGURES

Parameters for Fig. 4: $Z = 4$, $V = 0.5$, $t = 1.1$, $\delta t = 0.1$, $\varphi = 1.6\pi$, and

$$(r_v^1, r_v^2, r_v^3) = (0.417022, 0.720324, 0.000114) \quad , \quad \theta_v^n = -\frac{2\pi}{4} n \,, \tag{1}$$

$$(r_t^1, r_t^2, r_t^3) = (0.686260, 0.845561, 0.896767) \quad , \quad (\theta_t^1, \theta_t^2, \theta_t^3) = (3.385485, 5.267753, 0.349713) - \frac{2\pi}{4}(1,2,3) \,. \tag{2}$$

Parameters for Fig. 16(a): $Z = 6$, $V = 0.5$, $t = 1.$, $\delta t = 0.1$, and

$$(r_v^1, r_v^2, r_v^3) = (0.417022, 0.720324, 0.000114) \quad , \quad \theta_v^n = -\frac{2\pi}{6} n \,, \tag{3}$$

$$(r_t^1, r_t^2, r_t^3) = (0.686260, 0.845561, 0.896767) \quad , \quad (\theta_t^1, \theta_t^2, \theta_t^3) = (3.385485, 5.267753, 0.349713) - \frac{2\pi}{6}(1,2,3) \,. \tag{4}$$

Parameters for Fig. 16(b): $Z = 3$, $V = 0.5$, $t = 1.$, $\delta t = 0.$, and

$$(r_v^1, r_v^2, r_v^3, r_v^4, r_v^5) = (0.777702, 0.237541, 0.824279, 0.965749, 0.972601) \quad , \quad \theta_v^n = -\frac{2\pi}{3} n \,, \tag{5}$$

$$\tag{6}$$

Parameters for Fig. 18(a): $Z = 3$, $V = 0.1$, $t = 1.$, $\delta t = 0.1$, and

$$(v_1^{(0)}, v_2^{(0)}, v_3^{(0)}) = (0.06714, -0.03044, -0.03670) \quad , \quad (v_1^{(1)}, v_2^{(1)}, v_3^{(1)}) = (-0.22328, -0.00556, 0.22885) \tag{7}$$

$$(t_1^{(0)}, t_2^{(0)}, t_3^{(0)}) = (-0.25741, -0.22346, 0.39435) \quad , \quad (t_1^{(1)}, t_2^{(1)}, t_3^{(1)}) = (-0.25732, 0.22346, -0.29399) \,. \tag{8}$$

Parameters for Fig.18(b): $Z = 3$, $V = 0.1$, $t = 1.$, $\delta t = 0.1$, and

$$(v_1^{(0)}, v_2^{(0)}, v_3^{(0)}) = (0.06714, -0.03044, -0.03670) \quad , \quad (v_1^{(1)}, v_2^{(1)}, v_3^{(1)}) = (-0.41141, 0.14867, 0.26274) \tag{9}$$

$$(t_1^{(0)}, t_2^{(0)}, t_3^{(0)}) = (-0.25741, -0.22346, 0.39435) \quad , \quad (t_1^{(1)}, t_2^{(1)}, t_3^{(1)}) = (-0.25723, -0.32962, 0.01767) \,. \tag{10}$$

Parameters for Fig. 25(a-e): $Z = 4$, $V = 0.3$, $t = 1.$, $\delta t = 0.2$, and

$$(v_1^{(0)}, v_2^{(0)}, v_3^{(0)}, v_4^{(0)}) = (-0.032197, -0.061471, -0.063350, 0.157018, ) \cdot \frac{1}{0.3} \,,$$

$$(v_1^{(1)}, v_2^{(1)}, v_3^{(1)}, v_4^{(1)}) = (-0.028954, 0.027053, 0.038460, -0.036561) \cdot \frac{s}{0.3} \,, \tag{11}$$

$$(t_1^{(0)}, t_2^{(0)}, t_3^{(0)}, t_4^{(0)}) = (-0.038753, -0.031963, 0.091598, -0.020881) \cdot \frac{1}{0.2} \,,$$

$$(t_1^{(1)}, t_2^{(1)}, t_3^{(1)}, t_4^{(1)}) = (-0.009550, -0.016789, 0.017940, 0.008399) \cdot \frac{s}{0.2} \,, \tag{12}$$

where $s = 0$ for Fig. 25(a), $s = 0.5$ for Fig. 25(b), $s = 1$ for Fig. 25(c), $s = -0.5$ for Fig. 25(d), and $s = -1$ for Fig. 25(e).

## II. DETAILS ABOUT THE MOVIE IN THE SUPPLEMENTAL MATERIAL

Here we show snapshots of the movie shown in the supplemental material with the parameters following those of Fig. 5(a) in the main text. We use the same strategy as outline in [2] to highlight non-analyticities and plot the logarithm of the Cauchy-Riemann equation where we have replaced the derivatives by a finite difference.

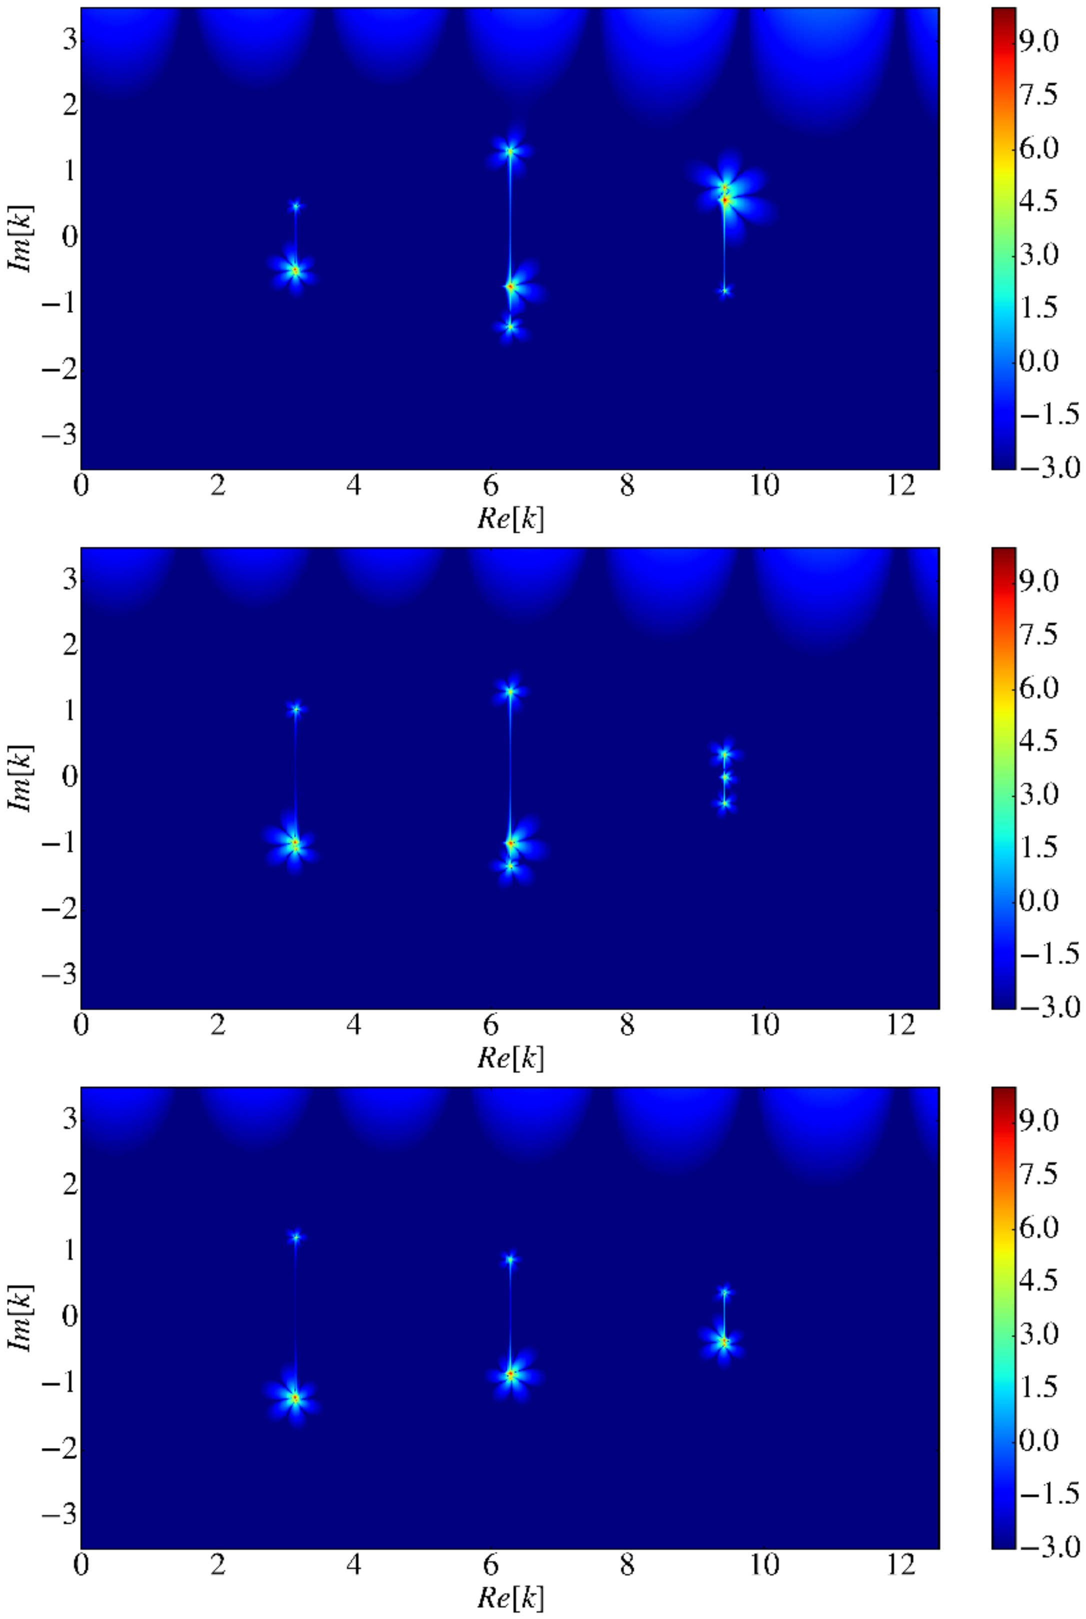


FIG. 1: From top to bottom: $\phi/\pi = 0, 0.1, 0.2$.

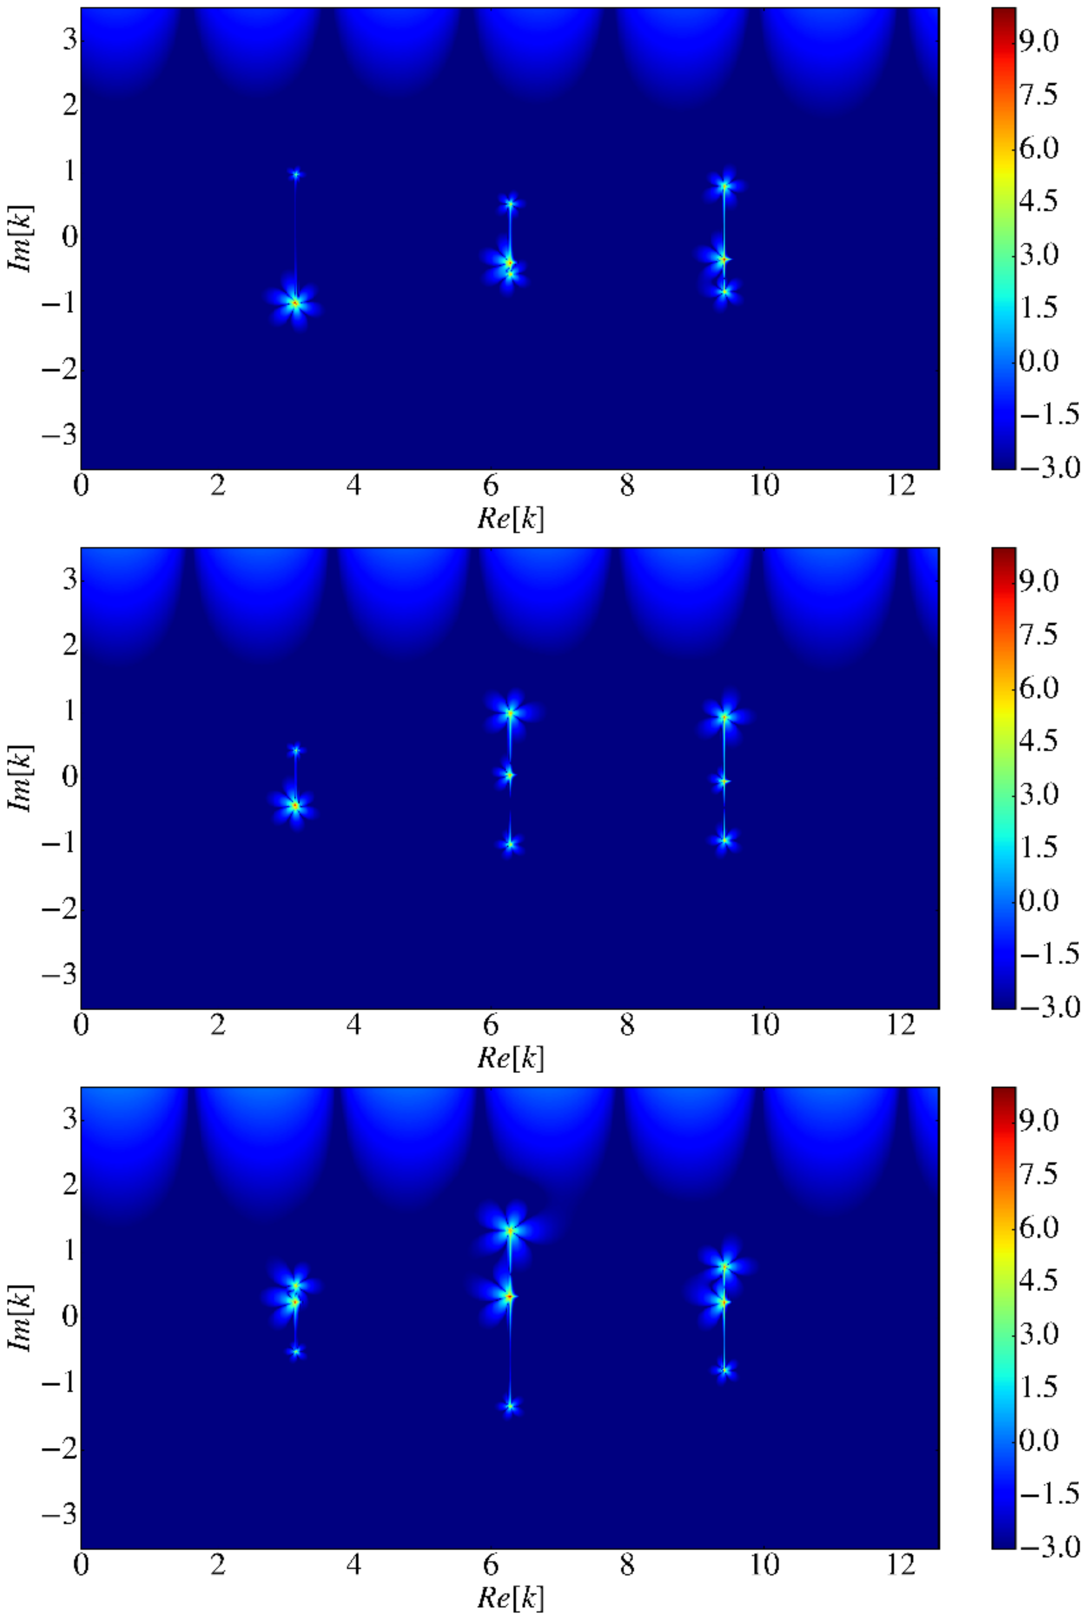


FIG. 2: From top to bottom: $\phi/\pi = 0.3, 0.4, 0.5$.

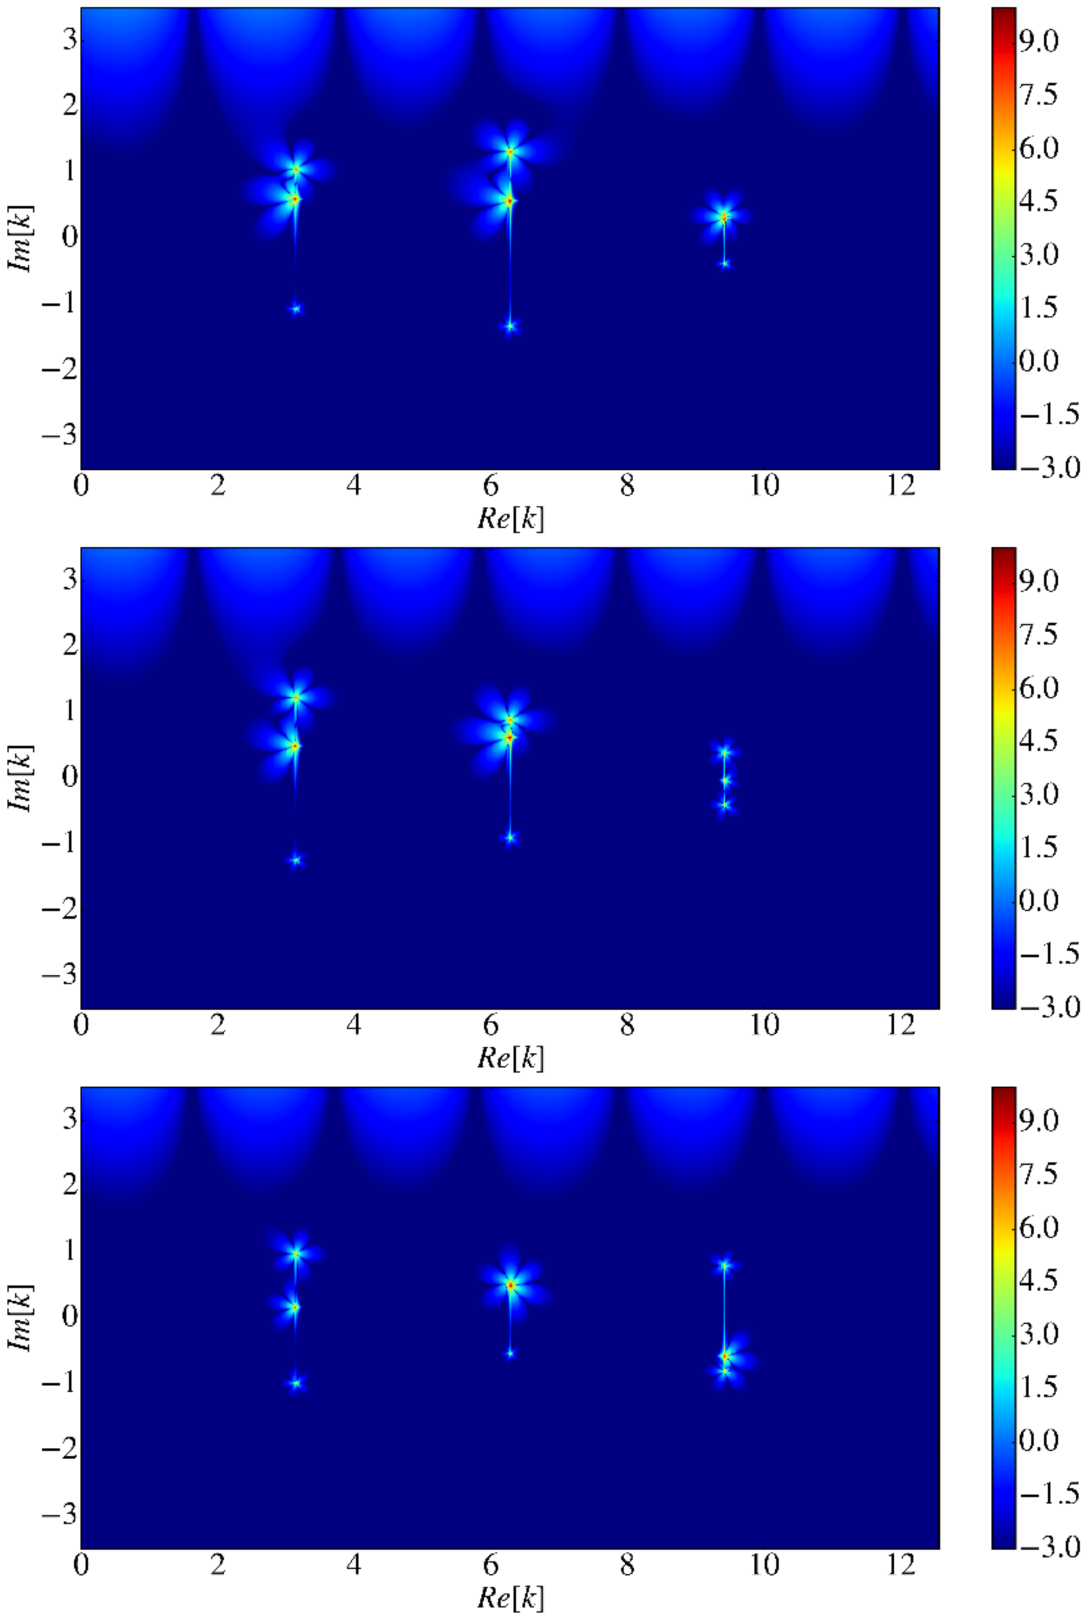


FIG. 3: From top to bottom: $\varphi/\pi = 0.6, 0.7, 0.8$

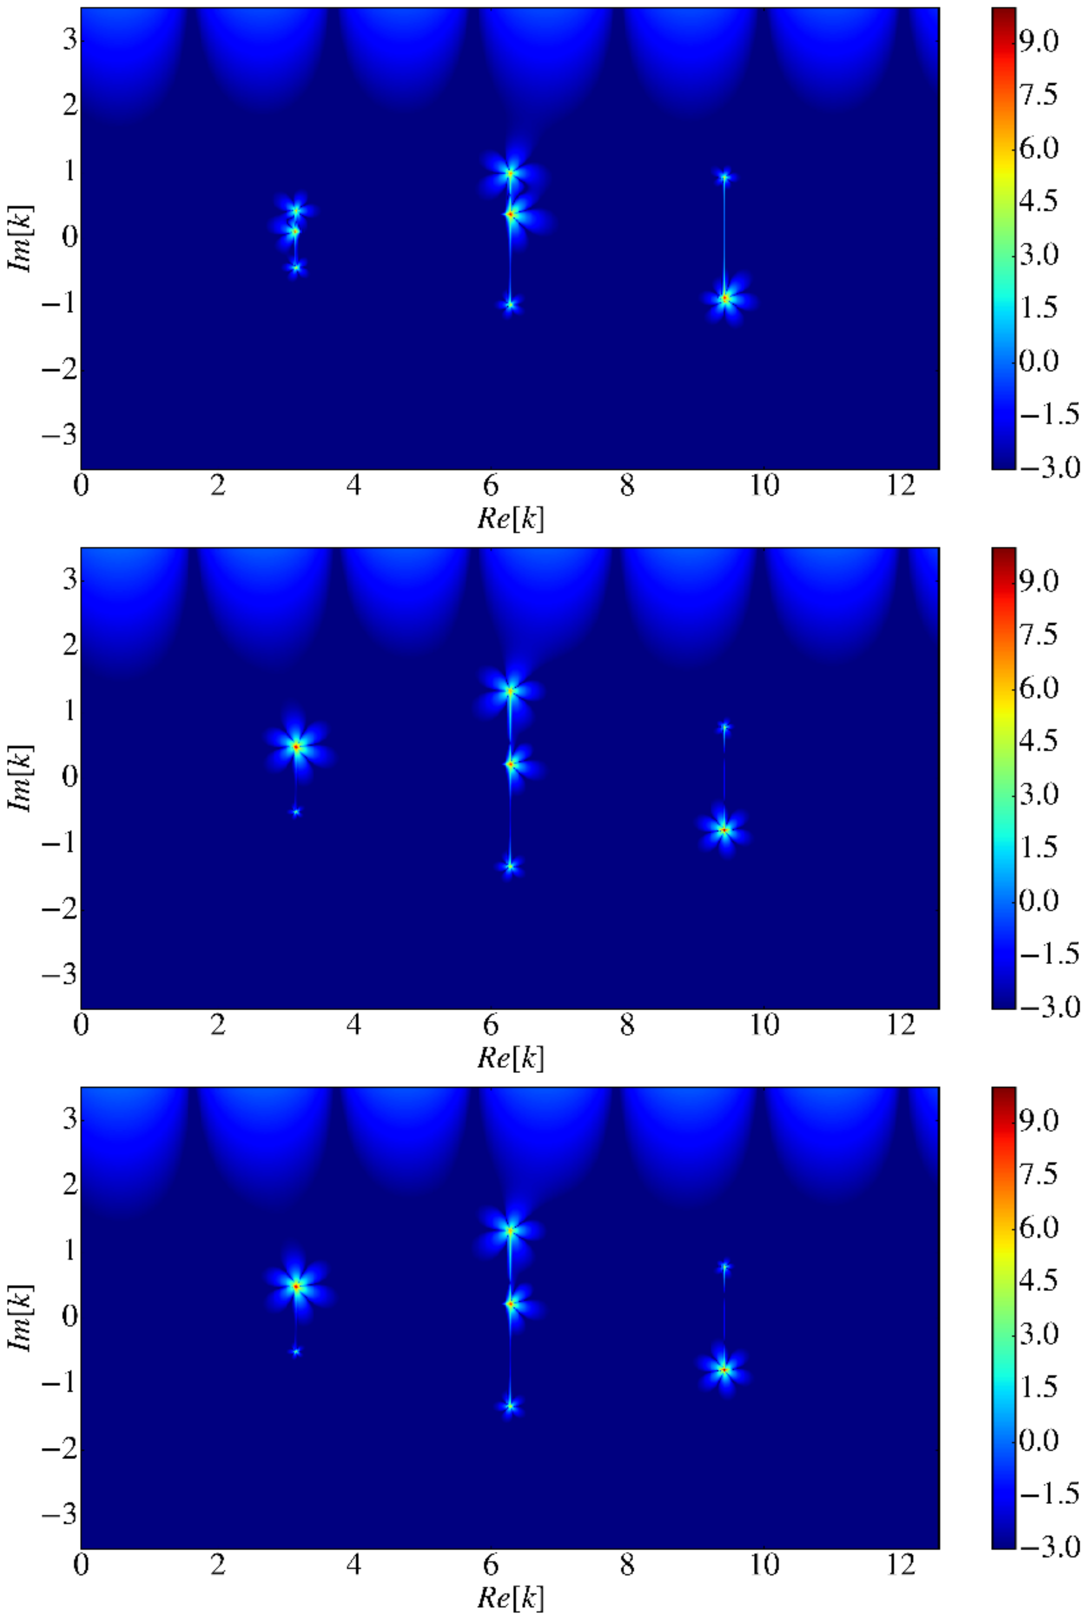


FIG. 4: From top to bottom: $\varphi/\pi = 0.9, 1.0, 1.1$

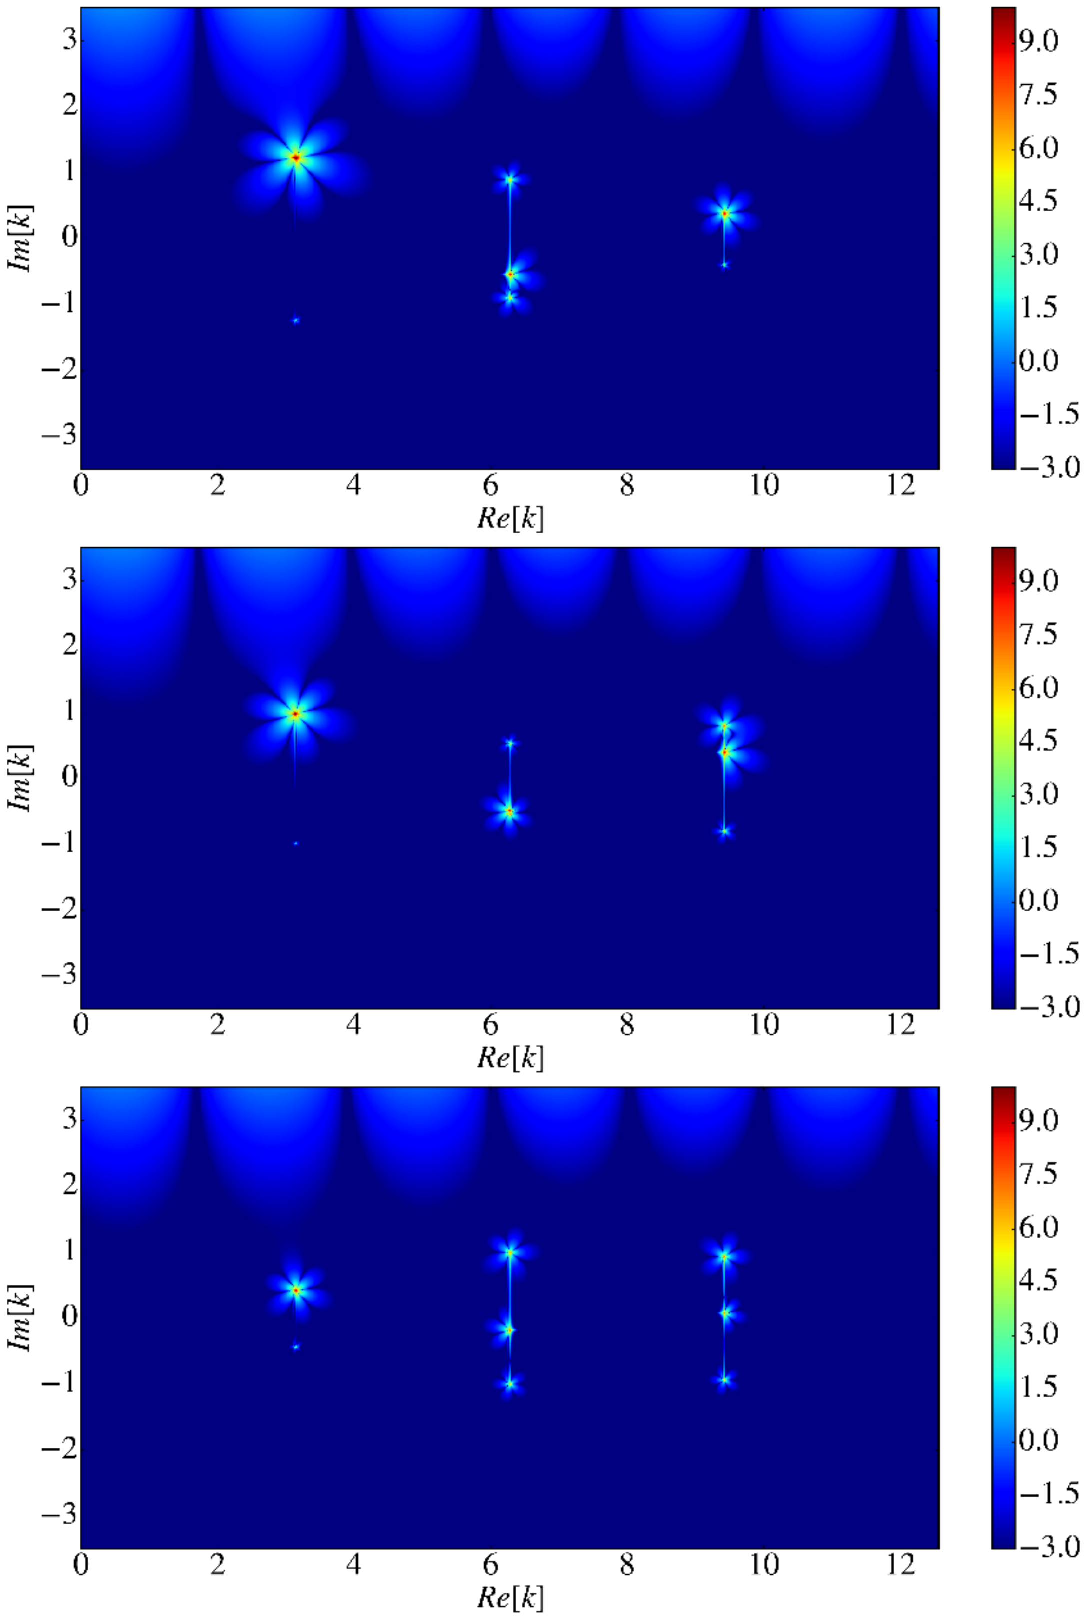


FIG. 5: From top to bottom: $\varphi/\pi = 1.2, 1.3, 1.4$

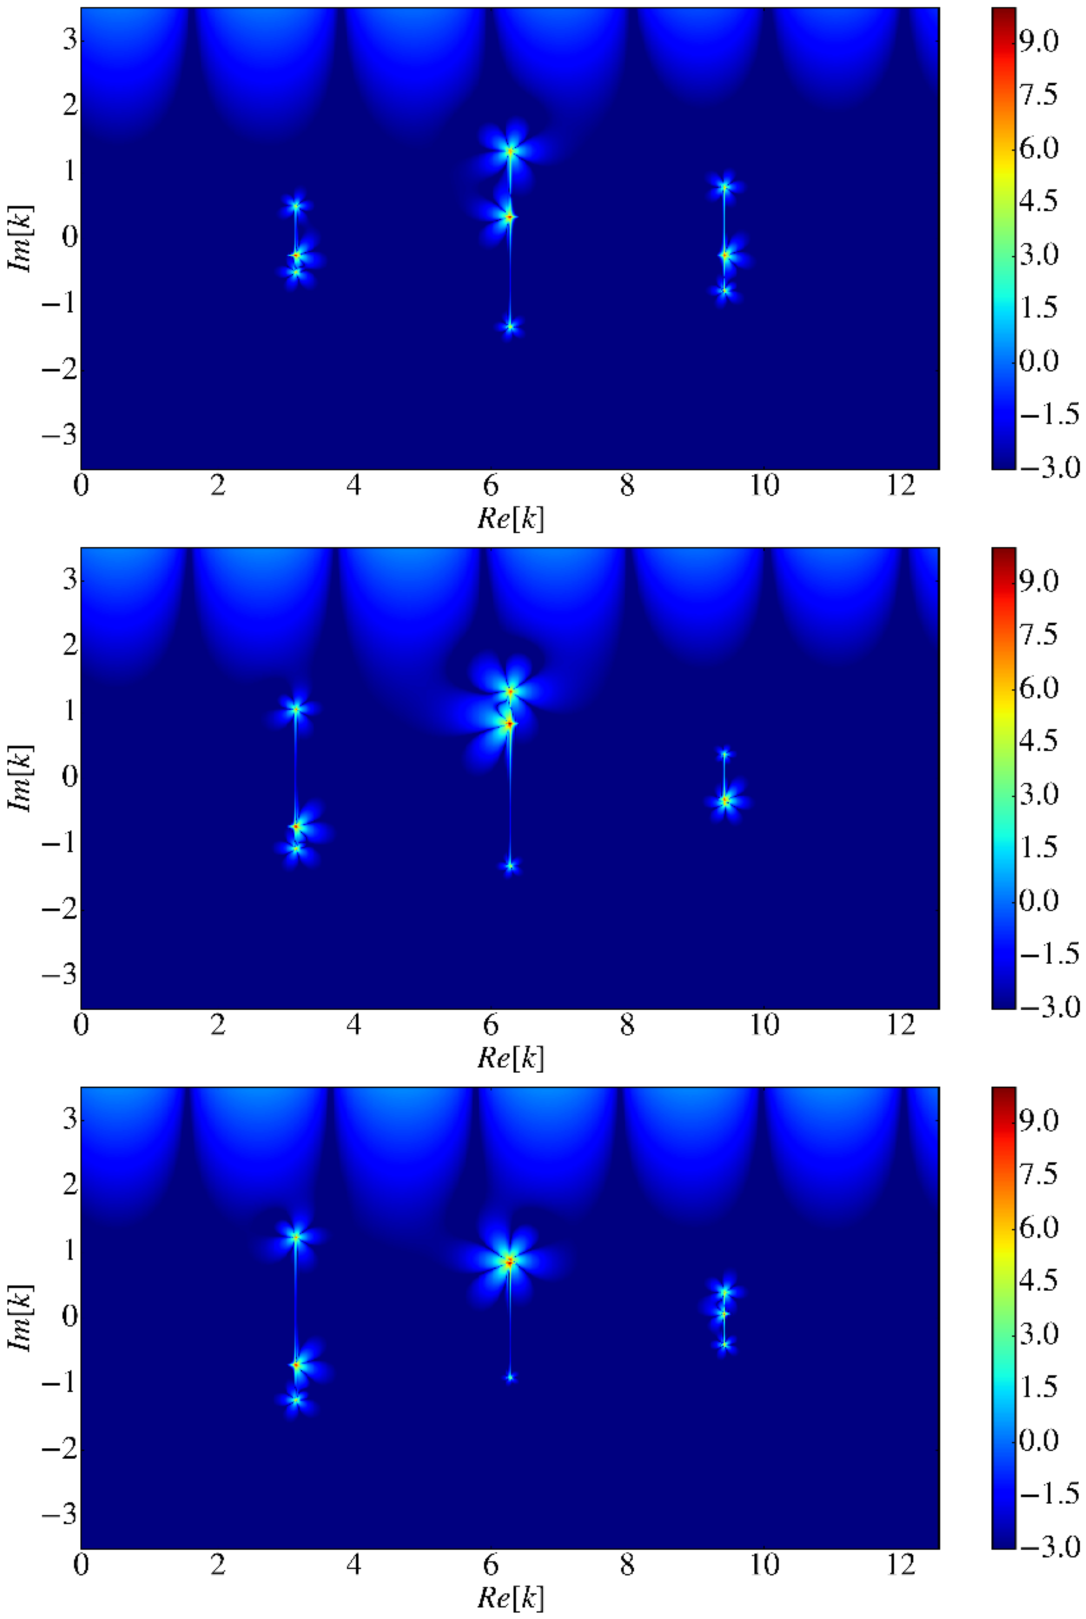


FIG. 6: From top to bottom: $\varphi/\pi = 1.5, 1.6, 1.7$.

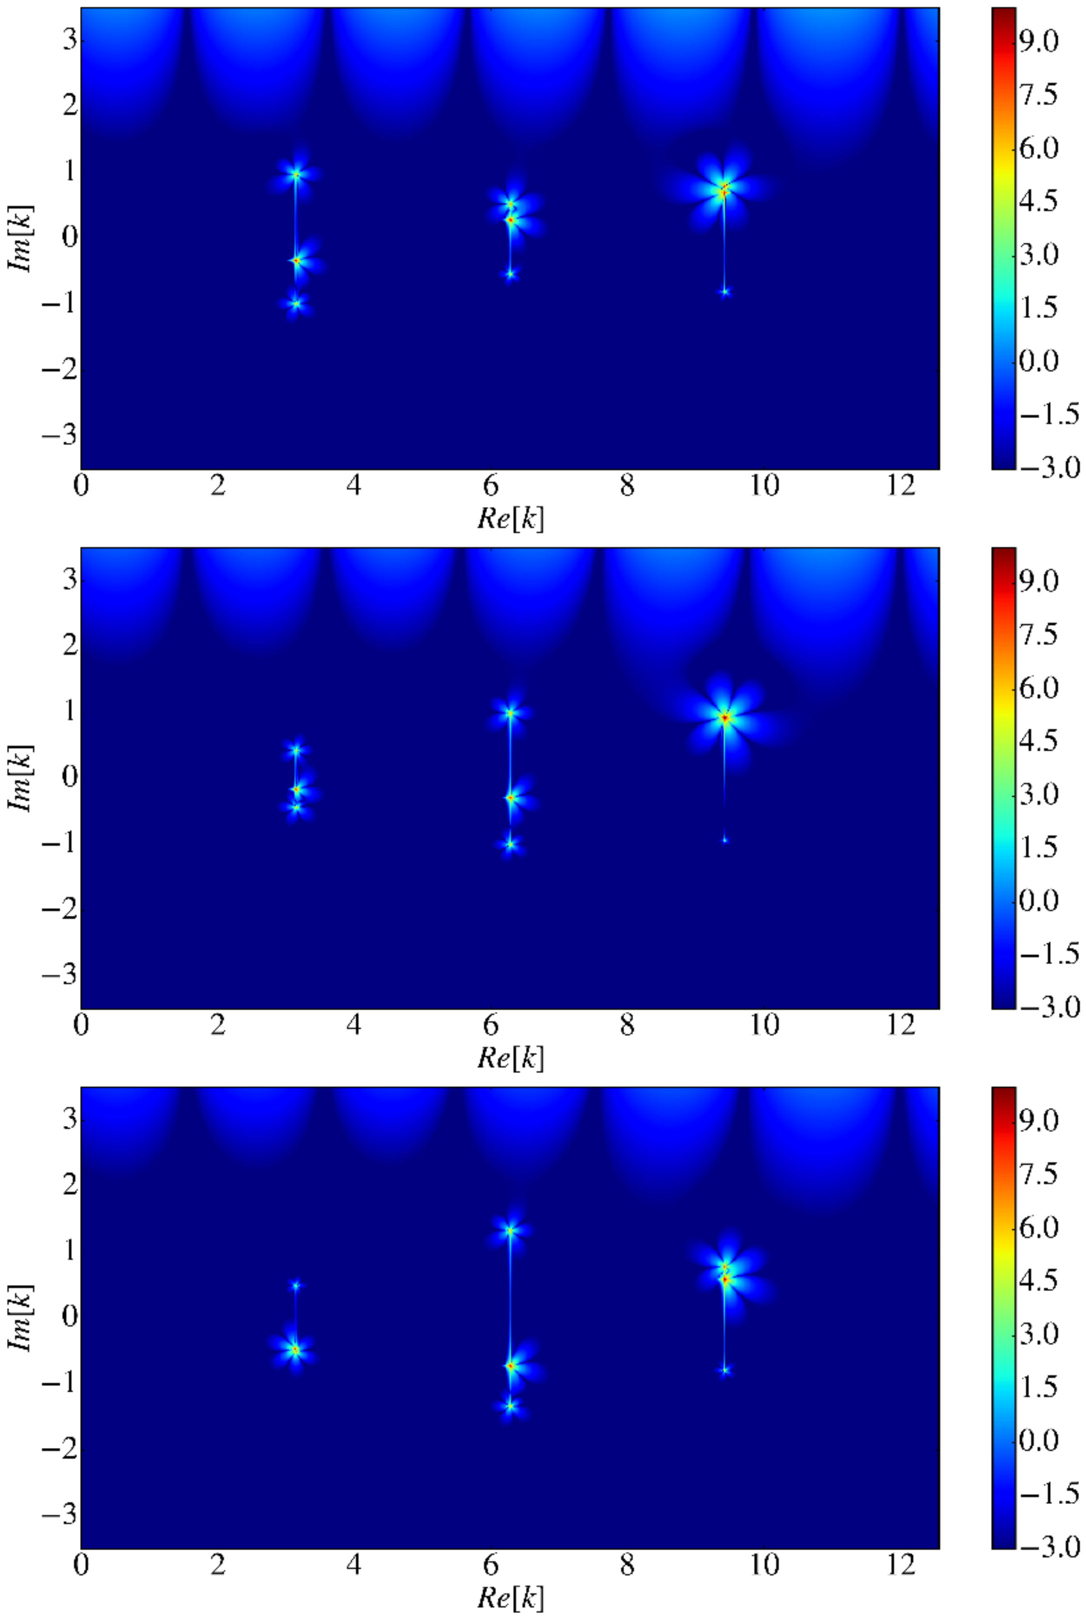


FIG. 7: From top to bottom: $\varphi/\pi = 1.8, 1.9, 2.0$.

* Email: schoeller@physik.rwth-aachen.de

[1] M. Pletyukhov, D.M. Kennes, J. Klinovaja, D. Loss, and H. Schoeller, submitted to Phys. Rev. B.
[2] D. M. Kennes, O. Kashuba, M. Pletyukhov, H. Schoeller, and V. Meden, Phys. Rev. Lett. **110**, 100405 (2013).
